# Supplementary material for: Evaluating Large Language Models for Stance Detection on Financial Targets from SEC Filing Reports and Earnings Call Transcripts
Source: arXiv:2510.23464 source file (2025-10-27)
Supplement: Supplementary file 1 [file supplementary.pdf]

## A LLM prompt for relevance filtering

```
message = [
{"role": "system",
"content": f"""You are a financial analyst. You are given a
sentence that is extracted from the quarterly earnings call
transcript of a company. Your task is to classify if the
sentence is relevant or not relevant to assess the company's
financial outlook towards targets "debt", "eps", or "sales"
from profitability perspective. The given sentence should
provide sufficient information to make the assessment without
needing external context."""},

{"role": "user",
"content": f"""# Task: Determine if the following sentence from
a company's quarterly earnings call is "relevant" or "not
relevant" for assessing the company's financial outlook
toward targets "debt", "eps", or "sales" from a profitability
perspective.

## Classify as 'relevant' if the sentence:

* Directly discusses performance, or outlook for the target.
* States a positive, negative, or neutral stance on the target.
* Contains projections or forward-looking statements about the
target.

## Classify as 'not relevant' if the sentence:

* Covers administrative, procedural, or logistical details
* Is a speaker introduction, general background, or technical
note
* Lacks sufficient information to determine the outlook for the
target
* Is a legal disclaimer, incomplete sentence, or out of context

**Instructions:**
For the sentence below, determine if the text is **relevant** or
**not relevant** for target "{target}". Also, give a short
reasoning for your classification.

Sentence: {text}
Relevance: [relevant / not relevant]
Reason: [Reasoning for the classification]"""}]
```

## B LLM prompt for stance annotation

```
message = [  
{"role": "user",  
"content": f"""  
You are a seasoned financial analyst reviewing individual  
sentences extracted from a company's SEC report. Your task is  
to determine the company's stance toward a specified  
financial target **{target}** from a profitability  
perspective. Classify each sentence as **Positive**,  
**Negative**, or **Neutral** based on the following criteria:
```

### Label Definitions:

- \* **Positive:** The sentence presents a favorable situation, trend, or outlook for the target **{target}** that positively impacts or supports the company's profitability. Examples include reduced debt levels, rising EPS, or increasing sales.
- \* **Negative:** The sentence portrays an unfavorable situation, trend, or outlook for the target **{target}**, negatively impacting or limiting the company's profitability. Examples include increasing debt burdens, declining EPS, or falling sales.
- \* **Neutral:** The sentence does not explicitly or implicitly reflect a clear stance or impact regarding the target **{target}**, either because it is not mentioned or because the stance is balanced or unclear.

### Analysis Guidelines:

1. **Focus specifically on mentions or implications related to the financial target—avoid general market or macroeconomic comments unless explicitly tied to the target.**
2. **Consider both direct references and contextual implications** (e.g., "revenue growth" implicitly refers to sales).
3. **Distinguish clearly between factual reporting and subjective evaluations**; both types may indicate a stance.
4. **Identify relevant financial cues and indicators**, such as:
  - \* Performance metrics: growth, stability, decline
  - \* Strategic financial decisions: refinancing, restructuring, capital allocation

- \* Risk assessments or warnings related to the target
  - \* Forward-looking statements, future projections, or company guidance
  - \* Comparative analysis: previous performance or industry benchmarks
5. **\*\*Evaluate conflicting or mixed signals\*\*** by determining the dominant or most contextually relevant stance.
  6. **\*\*If the target is neither directly mentioned nor indirectly implied\*\***, classify the stance as **\*\*Neutral\*\***.
  7. **\*\*Even a modest loss per diluted share is still perceived negatively\*\***

{transcript\_context}

The sentence for classification is given below:

- \* Sentence: {text}
- \* Target: {target}

Provide me the output below:

- \* Stance: [Positive / Negative / Neutral]
  - \* Explanation: [Brief justification of your classification based on the analysis guidelines]"""
- ]

## C Chain-of-Thought example

In this section, we present a few chain-of-thought (CoT) reasoning steps generated by the ChatGPT-o3-pro model on a few-shot examples selected from the training set. With the CoT prompt, we prompt LLM to think step-by-step and show the reasoning steps in *Chain-of-Thought Reasoning* section in the output. Examples below show the CoT outputs from the ChatGPT-o3-pro model.

### a) Dataset: SEC dataset (earnings per share (EPS))

Instance: *On an adjusted basis, net income attributable to 3M was \$5.088 billion, or \$8.74 per diluted share for 2020 compared to \$5.193 billion, or \$8.88 per diluted share in December 31, 2019, a decrease of 1.5 percent on a per diluted share basis.*

CoT Reasoning:

#### 1. Chain-of-Thought Reasoning

- The sentence explicitly discusses "\$8.74 per diluted share for 2020" versus "\$8.88 per diluted share in 2019," and says this is "a decrease of 1.5 percent."
- Per Guideline 4 (changes over time), a decline in EPS signals a deterioration in profitability.
- No offsetting positive cues are given, so the dominant context is the EPS decline.
- Therefore the stance toward EPS is Negative.
- The surrounding report data merely corroborate these figures; the sentence itself is sufficient, so the broader context is not necessary for classification.

#### 2. Stance: Negative

#### 3. Brief Justification: The sentence reports adjusted diluted EPS fell from \$8.88 to \$8.74, a 1.5% decrease, indicating weaker profitability.

### b) Dataset: ECT dataset (debt)

Instance: *all of our debt is prepayable without penalties or fees, and we're using excess cash flow to release borrowings against our revolving credit facility.*

CoT Reasoning:

#### 1. Chain-of-Thought Reasoning

- The sentence directly addresses debt management.
- "Debt is prepayable without penalties or fees" -> favorable terms; company can retire debt cheaply.
- "Using excess cash flow to release borrowings" -> actively paying down debt, lowering leverage and future interest expense.
- Lower interest expense and greater financial flexibility benefit profitability -> Positive stance.

#### 2. Stance: Positive

#### 3. Brief Justification: The sentence shows the company can repay debt inexpensively and is already reducing borrowings with excess cash, a clearly favorable situation for profitability.

## D Error Analysis

In this section, we do error analysis on the predictions from the LLMs (Llama3:70B). We first look at a few instances where the zero-shot setup makes an incorrect prediction, whereas the few-shot setup gets it correctly. We then look into the cases where the models fail without an explicit CoT prompt but succeed when CoT reasoning is included. Similarly, we look into situations where random examples fail, but similar examples help the model make a correct prediction.

### D.1 Zero-shot vs. Few-shot

1. Dataset: ECT dataset (debt)

Instance: *so with ebitda softer than we had anticipated this year reducing our leverage remains a top priority.*

Zero-shot prediction: Positive

Few-shot ( $k = 1$  prediction): Negative

Ground Truth (ChatGPT-o3-pro model): Negative

Reasoning from ChatGPT-o3-pro model:

1. Chain-of-Thought Reasoning
  - "EBITDA softer than we had anticipated" implies earnings have fallen, worsening the firm's leverage ratio.
  - Management says "reducing our leverage remains a top priority," signalling that current debt levels are viewed as too high and potentially harmful to profitability.
  - Emphasis on debt reduction reflects concern, not satisfaction, with the present debt situation. According to the guidelines, such concern over elevated debt is a Negative stance.
2. Stance: Negative
3. Brief Justification: The sentence states that weaker EBITDA has made lowering leverage a "top priority," indicating current debt levels are a problem for profitability.

### D.2 CoT vs. Non-CoT

1. Dataset: SEC dataset (sales)

Instance: *Research, Development and Related Expenses: R&D, measured as a percent of sales, decreased in 2022 when compared to the same period last year.*

Non-CoT prediction: Positive CoT prediction: Neutral

Ground-truth (ChatGPT-o3-pro model): Neutral

Reasoning from ChatGPT-o3-pro model:

1. Chain-of-Thought Reasoning
  - The only reference to "sales" is as the denominator in the R&D-to-sales ratio.

- The statement describes a change in R&D spending relative to sales but provides no information about whether sales themselves rose, fell, or remained flat.
  - Because it neither signals a favorable nor an unfavorable development specifically for sales, it fits guideline \#6: sales is only tangentially referenced -> Neutral.
2. Stance: Neutral
  3. Brief Justification: The sentence merely notes that R\&D expense as a percentage of sales declined, giving no clear indication of sales performance itself.

### **D.3 Random vs Similar example usage**

#### **1. Dataset: ECT**

Target: earnings per share (EPS)

Instance: we posted organic growth of 0.4% versus our expectation of 1% to 3%, along with adjusted margins of 19% and adjusted earnings of \$2.28 per share. Random example prediction: Positive Similar example prediction: Negative Ground-truth (ChatGPT-o3-pro model): Negative

Reasoning from ChatGPT-o3-pro model:

1. Chain-of-Thought Reasoning
  - The sentence compares actual results with management's expectations: organic growth came in at only 0.4% versus the 1%-3% that had been expected.
  - Falling short of internal expectations signals weaker performance and pressure on profitability.
  - Although it lists adjusted EPS of \$2.28, there is no positive comparison or improvement stated; the shortfall in growth is the dominant cue.
  - According to Guideline 5, when cues conflict, use the dominant context-in this case, the miss versus expectations-so the stance toward EPS is negative.
2. Stance: Negative
3. Brief Justification: The company delivered just 0.4% organic growth versus its 1%-3% target, implying weaker-than-expected earnings power and a negative outlook for EPS.

## E All experiment results

Table S1: Mean accuracy (% ,  $\pm$  standard deviation) of LLMs on the ECT and SEC datasets, evaluated using randomly selected few-shot examples under the No Transcript condition and without Chain-of-Thought (CoT) prompting. For each dataset, the highest score within each row is presented in bold. Results are averaged over three independent runs.

| Target | $k$ | ECT Data                           |                                    |                                    |                  | SEC Data                           |                                   |                                    |                  |
|--------|-----|------------------------------------|------------------------------------|------------------------------------|------------------|------------------------------------|-----------------------------------|------------------------------------|------------------|
|        |     | GPT-4.1-Mini                       | Gemma3:27B                         | Llama3.3:70B                       | Mistral:24B      | GPT-4.1-Mini                       | Gemma3:24B                        | Llama3.3:70B                       | Mistral:24B      |
| debt   | 0   | 85.57 $\pm$ 1.79                   | <b>87.29 <math>\pm</math> 0.6</b>  | 79.73 $\pm$ 3.31                   | 78.01 $\pm$ 6.86 | <b>85.91 <math>\pm</math> 0.6</b>  | 75.6 $\pm$ 0.6                    | 78.35 $\pm$ 1.79                   | 50.52 $\pm$ 3.57 |
|        | 1   | 83.51 $\pm$ 1.03                   | <b>86.6 <math>\pm</math> 0.0</b>   | 82.13 $\pm$ 2.15                   | 76.98 $\pm$ 1.19 | <b>82.47 <math>\pm</math> 1.79</b> | 75.26 $\pm$ 1.03                  | 73.2 $\pm$ 1.03                    | 54.3 $\pm$ 2.98  |
|        | 5   | 83.85 $\pm$ 0.6                    | <b>84.19 <math>\pm</math> 2.15</b> | <b>84.19 <math>\pm</math> 2.38</b> | 74.23 $\pm$ 1.79 | <b>81.79 <math>\pm</math> 0.6</b>  | 72.51 $\pm$ 0.6                   | 74.23 $\pm$ 1.03                   | 57.39 $\pm$ 2.15 |
|        | 10  | 81.44 $\pm$ 0.0                    | <b>86.25 <math>\pm</math> 0.6</b>  | 81.79 $\pm$ 2.38                   | 71.82 $\pm$ 2.38 | <b>80.07 <math>\pm</math> 0.6</b>  | 73.54 $\pm$ 1.19                  | 71.48 $\pm$ 2.15                   | 57.04 $\pm$ 2.38 |
| eps    | 0   | <b>88.5 <math>\pm</math> 0.68</b>  | 83.04 $\pm$ 0.0                    | 82.85 $\pm$ 1.47                   | 78.36 $\pm$ 0.58 | <b>80.18 <math>\pm</math> 1.56</b> | 68.47 $\pm$ 3.12                  | 72.07 $\pm$ 4.13                   | 60.36 $\pm$ 1.56 |
|        | 1   | <b>85.77 <math>\pm</math> 0.89</b> | 82.07 $\pm$ 0.34                   | 82.46 $\pm$ 1.55                   | 75.63 $\pm$ 2.36 | 75.68 $\pm$ 0.0                    | 65.77 $\pm$ 1.56                  | <b>77.48 <math>\pm</math> 3.12</b> | 55.86 $\pm$ 5.63 |
|        | 5   | <b>87.13 <math>\pm</math> 0.0</b>  | 81.29 $\pm$ 0.58                   | 82.65 $\pm$ 0.89                   | 73.29 $\pm$ 0.34 | <b>79.28 <math>\pm</math> 1.56</b> | 68.47 $\pm$ 1.56                  | 76.58 $\pm$ 1.56                   | 53.15 $\pm$ 3.12 |
|        | 10  | <b>85.38 <math>\pm</math> 1.01</b> | 84.21 $\pm$ 0.0                    | 81.87 $\pm$ 1.75                   | 74.07 $\pm$ 5.11 | <b>79.28 <math>\pm</math> 4.13</b> | 67.57 $\pm$ 0.0                   | 76.58 $\pm$ 1.56                   | 58.56 $\pm$ 4.13 |
| sales  | 0   | <b>92.2 <math>\pm</math> 0.34</b>  | 88.36 $\pm$ 0.2                    | 85.88 $\pm$ 1.99                   | 80.9 $\pm$ 2.15  | 91.62 $\pm$ 0.34                   | <b>92.2 <math>\pm</math> 0.34</b> | 89.08 $\pm$ 1.88                   | 78.36 $\pm$ 1.55 |
|        | 1   | <b>91.19 <math>\pm</math> 0.34</b> | 87.91 $\pm$ 0.71                   | 87.23 $\pm$ 1.74                   | 79.21 $\pm$ 1.67 | <b>91.81 <math>\pm</math> 0.58</b> | 89.86 $\pm$ 0.34                  | 86.74 $\pm$ 4.11                   | 76.41 $\pm$ 1.79 |
|        | 5   | <b>90.73 <math>\pm</math> 0.2</b>  | 88.93 $\pm$ 0.2                    | 89.15 $\pm$ 0.34                   | 80.34 $\pm$ 1.22 | <b>92.2 <math>\pm</math> 1.35</b>  | 87.33 $\pm$ 0.89                  | 88.3 $\pm$ 1.75                    | 74.27 $\pm$ 2.34 |
|        | 10  | <b>91.53 <math>\pm</math> 0.59</b> | 89.27 $\pm$ 0.2                    | 87.8 $\pm$ 2.69                    | 82.82 $\pm$ 2.82 | <b>90.25 <math>\pm</math> 0.34</b> | 88.69 $\pm$ 0.68                  | 87.72 $\pm$ 2.55                   | 77.19 $\pm$ 2.55 |

Table S2: Mean accuracy (% ,  $\pm$  standard deviation) of LLMs on the ECT and SEC datasets, evaluated using randomly selected few-shot examples under the No Transcript and Chain-of-Thought (CoT) prompting conditions. For each dataset, the highest score within each row is presented in bold. Results are averaged over three independent runs.

| Target | $k$ | ECT Data                           |                                    |                                    |                  | SEC Data                           |                                    |                                    |                  |
|--------|-----|------------------------------------|------------------------------------|------------------------------------|------------------|------------------------------------|------------------------------------|------------------------------------|------------------|
|        |     | GPT-4.1-Mini                       | Gemma3:27B                         | Llama3.3:70B                       | Mistral:24B      | GPT-4.1-Mini                       | Gemma3:24B                         | Llama3.3:70B                       | Mistral:24B      |
| debt   | 0   | 80.41 $\pm$ 3.72                   | 68.38 $\pm$ 1.57                   | <b>83.16 <math>\pm</math> 2.59</b> | 77.32 $\pm$ 2.06 | <b>82.47 <math>\pm</math> 3.72</b> | 69.42 $\pm$ 2.98                   | 78.35 $\pm$ 1.79                   | 72.85 $\pm$ 7.81 |
|        | 1   | 81.10 $\pm$ 2.38                   | 83.16 $\pm$ 3.15                   | <b>83.51 <math>\pm</math> 2.06</b> | 78.01 $\pm$ 5.68 | <b>82.47 <math>\pm</math> 2.73</b> | 79.38 $\pm$ 2.06                   | 78.69 $\pm$ 1.57                   | 72.51 $\pm$ 4.87 |
|        | 5   | <b>86.94 <math>\pm</math> 1.57</b> | 85.57 $\pm$ 1.79                   | 83.16 $\pm$ 1.57                   | 78.01 $\pm$ 5.29 | 81.79 $\pm$ 1.57                   | 82.82 $\pm$ 4.17                   | <b>83.16 <math>\pm</math> 3.62</b> | 65.64 $\pm$ 3.90 |
|        | 10  | <b>85.91 <math>\pm</math> 2.59</b> | 85.22 $\pm$ 3.31                   | 83.51 $\pm$ 0.0                    | 73.54 $\pm$ 6.55 | <b>84.54 <math>\pm</math> 2.06</b> | 83.85 $\pm$ 0.60                   | 82.82 $\pm$ 2.38                   | 75.26 $\pm$ 3.57 |
| eps    | 0   | <b>81.68 <math>\pm</math> 2.94</b> | 51.27 $\pm$ 0.68                   | 80.51 $\pm$ 1.88                   | 79.92 $\pm$ 2.88 | <b>87.39 <math>\pm</math> 4.13</b> | 45.05 $\pm$ 6.24                   | 72.97 $\pm$ 2.70                   | 71.17 $\pm$ 3.12 |
|        | 1   | <b>86.94 <math>\pm</math> 1.47</b> | 85.96 $\pm$ 0.58                   | 83.63 $\pm$ 1.17                   | 82.07 $\pm$ 2.64 | <b>91.89 <math>\pm</math> 5.41</b> | 74.77 $\pm$ 1.56                   | 79.28 $\pm$ 1.56                   | 63.96 $\pm$ 7.80 |
|        | 5   | <b>88.11 <math>\pm</math> 1.22</b> | 87.13 $\pm$ 1.01                   | 83.04 $\pm$ 2.03                   | 77.97 $\pm$ 1.22 | <b>88.29 <math>\pm</math> 3.12</b> | 69.37 $\pm$ 7.80                   | 78.38 $\pm$ 5.41                   | 74.77 $\pm$ 3.12 |
|        | 10  | <b>85.58 <math>\pm</math> 2.21</b> | <b>85.58 <math>\pm</math> 2.05</b> | 84.21 $\pm$ 0.58                   | 80.51 $\pm$ 1.47 | <b>85.59 <math>\pm</math> 4.13</b> | 70.27 $\pm$ 0.0                    | 72.07 $\pm$ 1.56                   | 72.97 $\pm$ 2.70 |
| sales  | 0   | 78.98 $\pm$ 5.33                   | 62.60 $\pm$ 3.41                   | <b>87.34 <math>\pm</math> 1.28</b> | 83.73 $\pm$ 1.55 | 84.60 $\pm$ 1.79                   | 63.94 $\pm$ 3.00                   | <b>91.03 <math>\pm</math> 0.68</b> | 84.21 $\pm$ 3.56 |
|        | 1   | <b>92.54 <math>\pm</math> 1.17</b> | 90.96 $\pm$ 0.71                   | 90.62 $\pm$ 1.74                   | 85.42 $\pm$ 2.37 | <b>90.25 <math>\pm</math> 2.43</b> | <b>90.25 <math>\pm</math> 0.34</b> | <b>90.25 <math>\pm</math> 0.89</b> | 84.02 $\pm$ 1.47 |
|        | 5   | <b>92.54 <math>\pm</math> 1.36</b> | 90.06 $\pm$ 0.85                   | 90.73 $\pm$ 0.52                   | 82.82 $\pm$ 1.67 | 88.30 $\pm$ 2.11                   | <b>89.47 <math>\pm</math> 1.55</b> | 88.50 $\pm$ 1.22                   | 80.90 $\pm$ 1.88 |
|        | 10  | <b>92.66 <math>\pm</math> 0.71</b> | 91.41 $\pm$ 0.71                   | 89.72 $\pm$ 0.52                   | 83.84 $\pm$ 1.41 | <b>90.25 <math>\pm</math> 0.68</b> | 88.30 $\pm$ 0.58                   | 88.89 $\pm$ 1.55                   | 82.85 $\pm$ 1.47 |

Table S3: Mean accuracy (% ,  $\pm$  standard deviation) of LLMs on the ECT and SEC datasets, evaluated using randomly selected few-shot examples under Full Transcript prompting without Chain-of-Thought (CoT). For each dataset, the highest score within each row is presented in bold. Results are averaged over three independent runs.

| Target | $k$ | ECT Data                           |                  |                  |                  | SEC Data                           |                  |                  |                  |
|--------|-----|------------------------------------|------------------|------------------|------------------|------------------------------------|------------------|------------------|------------------|
|        |     | GPT-4.1-Mini                       | Gemma3:27B       | Llama3.3:70B     | Mistral:24B      | GPT-4.1-Mini                       | Gemma3:24B       | Llama3.3:70B     | Mistral:24B      |
| debt   | 0   | <b>92.10 <math>\pm</math> 0.60</b> | 84.19 $\pm$ 1.57 | 87.63 $\pm$ 2.73 | 40.89 $\pm$ 2.38 | <b>82.82 <math>\pm</math> 0.60</b> | 57.39 $\pm$ 1.19 | 55.33 $\pm$ 0.60 | 25.09 $\pm$ 1.57 |
|        | 1   | <b>89.35 <math>\pm</math> 0.60</b> | 79.73 $\pm$ 1.57 | 86.94 $\pm$ 3.62 | 41.92 $\pm$ 3.15 | <b>79.73 <math>\pm</math> 1.57</b> | 62.54 $\pm$ 1.57 | 59.79 $\pm$ 2.06 | 28.18 $\pm$ 2.15 |
|        | 5   | <b>89.69 <math>\pm</math> 1.79</b> | 83.85 $\pm$ 0.60 | 84.54 $\pm$ 1.79 | 45.02 $\pm$ 5.68 | <b>79.38 <math>\pm</math> 1.03</b> | 64.60 $\pm$ 1.57 | 56.36 $\pm$ 2.15 | 33.33 $\pm$ 0.60 |
|        | 10  | <b>91.41 <math>\pm</math> 0.60</b> | 83.51 $\pm$ 0.00 | 84.54 $\pm$ 3.09 | 46.05 $\pm$ 1.19 | <b>80.41 <math>\pm</math> 0.00</b> | 65.64 $\pm$ 1.57 | 55.33 $\pm$ 0.60 | 36.08 $\pm$ 2.06 |
| eps    | 0   | <b>87.52 <math>\pm</math> 0.68</b> | 86.74 $\pm$ 1.22 | 86.74 $\pm$ 2.21 | 63.74 $\pm$ 1.55 | <b>81.08 <math>\pm</math> 0.00</b> | 65.77 $\pm$ 1.56 | 65.77 $\pm$ 1.56 | 44.14 $\pm$ 8.26 |
|        | 1   | <b>89.08 <math>\pm</math> 0.68</b> | 87.91 $\pm$ 1.35 | 86.16 $\pm$ 2.43 | 65.50 $\pm$ 1.55 | <b>81.08 <math>\pm</math> 0.00</b> | 70.27 $\pm$ 0.00 | 64.86 $\pm$ 0.00 | 56.76 $\pm$ 7.15 |
|        | 5   | <b>89.47 <math>\pm</math> 0.58</b> | 84.80 $\pm$ 1.55 | 85.96 $\pm$ 2.11 | 64.52 $\pm$ 0.68 | <b>81.08 <math>\pm</math> 0.00</b> | 69.37 $\pm$ 1.56 | 63.06 $\pm$ 4.13 | 47.75 $\pm$ 3.12 |
|        | 10  | <b>90.25 <math>\pm</math> 0.34</b> | 85.19 $\pm$ 0.89 | 83.43 $\pm$ 2.05 | 67.06 $\pm$ 2.05 | <b>79.28 <math>\pm</math> 1.56</b> | 66.67 $\pm$ 4.13 | 63.96 $\pm$ 3.12 | 57.66 $\pm$ 4.13 |
| sales  | 0   | <b>92.77 <math>\pm</math> 0.20</b> | 89.38 $\pm$ 0.52 | 89.49 $\pm$ 1.76 | 64.07 $\pm$ 2.35 | <b>91.62 <math>\pm</math> 1.22</b> | 85.38 $\pm$ 1.75 | 87.52 $\pm$ 0.89 | 57.31 $\pm$ 0.58 |
|        | 1   | <b>93.90 <math>\pm</math> 0.59</b> | 89.72 $\pm$ 0.71 | 88.47 $\pm$ 1.79 | 66.78 $\pm$ 1.89 | <b>92.59 <math>\pm</math> 0.34</b> | 88.69 $\pm$ 0.89 | 87.91 $\pm$ 0.89 | 71.15 $\pm$ 4.15 |
|        | 5   | <b>94.35 <math>\pm</math> 0.52</b> | 88.47 $\pm$ 0.34 | 88.70 $\pm$ 1.87 | 70.40 $\pm$ 2.21 | <b>90.25 <math>\pm</math> 0.89</b> | 86.55 $\pm$ 2.34 | 86.16 $\pm$ 1.88 | 64.91 $\pm$ 1.55 |
|        | 10  | <b>92.66 <math>\pm</math> 0.85</b> | 88.59 $\pm$ 1.04 | 87.46 $\pm$ 0.59 | 67.12 $\pm$ 0.90 | <b>89.86 <math>\pm</math> 0.34</b> | 84.60 $\pm$ 3.71 | 86.16 $\pm$ 2.76 | 66.08 $\pm$ 3.26 |

Table S4: Mean accuracy (% ,  $\pm$  standard deviation) of LLMs on the ECT and SEC datasets, evaluated using randomly selected few-shot examples under Full Transcript with Chain-of-Thought (CoT) prompting conditions. For each dataset, the highest score within each row is presented in bold. Results are averaged over three independent runs.

| Target | $k$ | ECT Data                           |                  |                                    |                  | SEC Data                           |                                    |                                    |                  |
|--------|-----|------------------------------------|------------------|------------------------------------|------------------|------------------------------------|------------------------------------|------------------------------------|------------------|
|        |     | GPT-4.1-Mini                       | Gemma3:27B       | Llama3.3:70B                       | Mistral:24B      | GPT-4.1-Mini                       | Gemma3:24B                         | Llama3.3:70B                       | Mistral:24B      |
| debt   | 0   | <b>90.03 <math>\pm</math> 1.57</b> | 80.07 $\pm$ 2.59 | 84.88 $\pm$ 2.15                   | 50.86 $\pm$ 2.15 | 75.60 $\pm$ 3.15                   | 67.35 $\pm$ 1.57                   | <b>78.01 <math>\pm</math> 1.57</b> | 34.71 $\pm$ 4.65 |
|        | 1   | <b>91.07 <math>\pm</math> 2.38</b> | 85.91 $\pm$ 1.57 | 84.54 $\pm$ 1.79                   | 81.10 $\pm$ 3.90 | 76.98 $\pm$ 4.65                   | <b>78.01 <math>\pm</math> 1.57</b> | <b>78.01 <math>\pm</math> 4.17</b> | 68.38 $\pm$ 0.60 |
|        | 5   | <b>92.10 <math>\pm</math> 2.59</b> | 84.54 $\pm$ 3.72 | 87.29 $\pm$ 3.15                   | 78.01 $\pm$ 5.19 | <b>81.10 <math>\pm</math> 1.57</b> | <b>81.10 <math>\pm</math> 1.57</b> | 78.69 $\pm$ 2.15                   | 69.42 $\pm$ 2.38 |
|        | 10  | <b>92.44 <math>\pm</math> 0.60</b> | 85.91 $\pm$ 1.19 | 87.63 $\pm$ 3.72                   | 75.60 $\pm$ 1.19 | <b>81.44 <math>\pm</math> 2.73</b> | 80.76 $\pm$ 2.15                   | 79.73 $\pm$ 1.57                   | 74.23 $\pm$ 2.73 |
| eps    | 0   | <b>85.77 <math>\pm</math> 1.79</b> | 81.09 $\pm$ 0.89 | 85.19 $\pm$ 1.79                   | 56.53 $\pm$ 2.36 | <b>78.38 <math>\pm</math> 7.15</b> | 59.46 $\pm$ 5.41                   | 68.47 $\pm$ 3.12                   | 39.64 $\pm$ 1.56 |
|        | 1   | <b>91.81 <math>\pm</math> 1.75</b> | 88.11 $\pm$ 0.89 | 85.96 $\pm$ 2.68                   | 79.53 $\pm$ 1.17 | <b>90.99 <math>\pm</math> 1.56</b> | 73.87 $\pm$ 3.12                   | 72.07 $\pm$ 4.13                   | 68.47 $\pm$ 4.13 |
|        | 5   | <b>89.28 <math>\pm</math> 1.69</b> | 86.35 $\pm$ 0.34 | 85.96 $\pm$ 2.34                   | 79.14 $\pm$ 1.47 | <b>87.39 <math>\pm</math> 6.80</b> | 77.48 $\pm$ 3.12                   | 75.68 $\pm$ 2.70                   | 66.67 $\pm$ 1.56 |
|        | 10  | <b>88.69 <math>\pm</math> 0.89</b> | 86.94 $\pm$ 0.68 | 85.19 $\pm$ 1.79                   | 80.70 $\pm$ 1.55 | <b>88.29 <math>\pm</math> 4.13</b> | 72.97 $\pm$ 2.70                   | 77.48 $\pm$ 3.12                   | 68.47 $\pm$ 1.56 |
| sales  | 0   | 90.17 $\pm$ 1.79                   | 81.58 $\pm$ 2.76 | <b>90.62 <math>\pm</math> 1.28</b> | 67.12 $\pm$ 1.22 | <b>89.47 <math>\pm</math> 1.17</b> | 67.84 $\pm$ 2.55                   | 88.89 $\pm$ 1.55                   | 59.45 $\pm$ 4.11 |
|        | 1   | <b>94.24 <math>\pm</math> 1.48</b> | 91.19 $\pm$ 1.02 | 88.93 $\pm$ 1.04                   | 87.12 $\pm$ 1.17 | <b>90.25 <math>\pm</math> 0.89</b> | 89.08 $\pm$ 1.88                   | 87.13 $\pm$ 2.11                   | 84.21 $\pm$ 2.11 |
|        | 5   | <b>94.12 <math>\pm</math> 1.37</b> | 90.51 $\pm$ 0.90 | 89.49 $\pm$ 1.17                   | 85.08 $\pm$ 1.36 | <b>91.03 <math>\pm</math> 1.47</b> | 89.28 $\pm$ 1.79                   | 84.60 $\pm$ 1.47                   | 83.24 $\pm$ 0.68 |
|        | 10  | <b>94.24 <math>\pm</math> 1.22</b> | 91.19 $\pm$ 0.34 | 89.83 $\pm$ 2.12                   | 84.41 $\pm$ 1.02 | <b>90.06 <math>\pm</math> 1.75</b> | <b>90.06 <math>\pm</math> 0.00</b> | 85.96 $\pm$ 1.75                   | 82.85 $\pm$ 1.47 |

Table S5: Mean accuracy (% ,  $\pm$  standard deviation) of LLMs on the ECT and SEC datasets, evaluated using randomly selected few-shot examples under Summarized Transcript prompting without Chain-of-Thought (CoT). For each dataset, the highest score within each row is presented in bold. Results are averaged over three independent runs.

| Target | $k$ | ECT Data                           |                  |                  |                  | SEC Data                           |                  |                                    |                  |
|--------|-----|------------------------------------|------------------|------------------|------------------|------------------------------------|------------------|------------------------------------|------------------|
|        |     | GPT-4.1-Mini                       | Gemma3:27B       | Llama3.3:70B     | Mistral:24B      | GPT-4.1-Mini                       | Gemma3:24B       | Llama3.3:70B                       | Mistral:24B      |
| debt   | 0   | <b>90.38 <math>\pm</math> 0.60</b> | 88.32 $\pm$ 0.60 | 84.19 $\pm$ 4.76 | 76.98 $\pm$ 0.60 | <b>82.47 <math>\pm</math> 1.03</b> | 71.82 $\pm$ 0.60 | 75.60 $\pm$ 2.15                   | 21.31 $\pm$ 2.15 |
|        | 1   | <b>90.03 <math>\pm</math> 0.60</b> | 87.29 $\pm$ 1.57 | 87.29 $\pm$ 0.60 | 69.42 $\pm$ 2.98 | <b>84.54 <math>\pm</math> 1.03</b> | 70.45 $\pm$ 2.15 | 71.82 $\pm$ 1.57                   | 21.99 $\pm$ 2.15 |
|        | 5   | <b>88.66 <math>\pm</math> 1.03</b> | 82.13 $\pm$ 0.60 | 85.22 $\pm$ 3.31 | 61.51 $\pm$ 3.62 | <b>82.13 <math>\pm</math> 0.60</b> | 67.70 $\pm$ 1.57 | 79.04 $\pm$ 2.15                   | 30.58 $\pm$ 0.60 |
|        | 10  | <b>88.66 <math>\pm</math> 1.03</b> | 84.88 $\pm$ 1.19 | 85.22 $\pm$ 4.17 | 55.33 $\pm$ 3.15 | <b>82.13 <math>\pm</math> 0.60</b> | 69.42 $\pm$ 0.60 | 80.76 $\pm$ 2.59                   | 36.43 $\pm$ 2.15 |
| eps    | 0   | <b>88.69 <math>\pm</math> 0.34</b> | 84.02 $\pm$ 0.89 | 85.38 $\pm$ 1.17 | 71.93 $\pm$ 3.09 | <b>81.08 <math>\pm</math> 2.70</b> | 69.37 $\pm$ 4.13 | 67.57 $\pm$ 4.68                   | 40.54 $\pm$ 5.41 |
|        | 1   | <b>87.33 <math>\pm</math> 0.68</b> | 84.99 $\pm$ 0.34 | 84.60 $\pm$ 2.05 | 68.42 $\pm$ 3.26 | <b>81.98 <math>\pm</math> 1.56</b> | 70.27 $\pm$ 2.70 | 74.77 $\pm$ 1.56                   | 45.95 $\pm$ 2.70 |
|        | 5   | <b>87.52 <math>\pm</math> 0.34</b> | 85.77 $\pm$ 0.34 | 84.80 $\pm$ 2.55 | 65.50 $\pm$ 1.75 | <b>84.68 <math>\pm</math> 1.56</b> | 63.06 $\pm$ 4.13 | 75.68 $\pm$ 2.70                   | 51.35 $\pm$ 2.70 |
|        | 10  | <b>87.72 <math>\pm</math> 0.00</b> | 85.38 $\pm$ 0.00 | 84.80 $\pm$ 1.17 | 66.86 $\pm$ 1.47 | <b>81.98 <math>\pm</math> 1.56</b> | 69.37 $\pm$ 6.24 | 72.07 $\pm$ 1.56                   | 53.15 $\pm$ 3.12 |
| sales  | 0   | <b>93.22 <math>\pm</math> 0.68</b> | 89.83 $\pm$ 0.68 | 88.59 $\pm$ 2.54 | 74.01 $\pm$ 2.07 | <b>92.40 <math>\pm</math> 0.58</b> | 87.91 $\pm$ 1.88 | 89.86 $\pm$ 2.36                   | 45.81 $\pm$ 3.38 |
|        | 1   | <b>93.11 <math>\pm</math> 0.52</b> | 90.62 $\pm$ 0.52 | 87.80 $\pm$ 2.94 | 71.30 $\pm$ 1.57 | <b>91.42 <math>\pm</math> 1.47</b> | 90.64 $\pm$ 1.17 | <b>91.42 <math>\pm</math> 2.88</b> | 55.17 $\pm$ 0.89 |
|        | 5   | <b>93.90 <math>\pm</math> 0.00</b> | 90.40 $\pm$ 0.39 | 88.59 $\pm$ 2.59 | 68.70 $\pm$ 0.52 | <b>91.62 <math>\pm</math> 0.34</b> | 87.13 $\pm$ 1.55 | <b>91.62 <math>\pm</math> 2.76</b> | 57.12 $\pm$ 2.88 |
|        | 10  | <b>93.90 <math>\pm</math> 0.34</b> | 90.85 $\pm$ 0.68 | 88.81 $\pm$ 2.90 | 67.80 $\pm$ 1.89 | 90.45 $\pm$ 0.68                   | 89.28 $\pm$ 0.89 | <b>92.40 <math>\pm</math> 0.58</b> | 64.13 $\pm$ 2.43 |

Table S6: Mean accuracy (% ,  $\pm$  standard deviation) of LLMs on the ECT and SEC datasets, evaluated using randomly selected few-shot examples under Summarized Transcript with Chain-of-Thought (CoT) prompting conditions. For each dataset, the highest score within each row is presented in bold. Results are averaged over three independent runs.

| Target | $k$ | ECT Data                           |                  |                                    |                  | SEC Data                           |                                    |                                    |                   |
|--------|-----|------------------------------------|------------------|------------------------------------|------------------|------------------------------------|------------------------------------|------------------------------------|-------------------|
|        |     | GPT-4.1-Mini                       | Gemma3:27B       | Llama3.3:70B                       | Mistral:24B      | GPT-4.1-Mini                       | Gemma3:24B                         | Llama3.3:70B                       | Mistral:24B       |
| debt   | 0   | 87.29 $\pm$ 2.59                   | 78.69 $\pm$ 2.59 | <b>88.32 <math>\pm</math> 1.19</b> | 79.73 $\pm$ 2.15 | 77.66 $\pm$ 2.15                   | 66.32 $\pm$ 1.57                   | <b>81.44 <math>\pm</math> 4.72</b> | 38.14 $\pm$ 4.72  |
|        | 1   | <b>89.0 <math>\pm</math> 2.98</b>  | 86.6 $\pm$ 1.03  | 85.57 $\pm$ 2.06                   | 79.04 $\pm$ 8.27 | 79.38 $\pm$ 2.06                   | 80.41 $\pm$ 1.79                   | <b>81.1 <math>\pm</math> 2.38</b>  | 70.45 $\pm$ 4.29  |
|        | 5   | 87.97 $\pm$ 2.59                   | 85.22 $\pm$ 2.59 | <b>88.32 <math>\pm</math> 1.57</b> | 77.66 $\pm$ 1.57 | <b>82.47 <math>\pm</math> 1.03</b> | 82.13 $\pm$ 1.19                   | 82.13 $\pm$ 0.6                    | 68.73 $\pm$ 3.31  |
|        | 10  | <b>86.94 <math>\pm</math> 3.62</b> | 84.19 $\pm$ 2.15 | 83.85 $\pm$ 0.6                    | 76.29 $\pm$ 3.57 | <b>84.19 <math>\pm</math> 2.15</b> | 80.41 $\pm$ 2.73                   | 81.79 $\pm$ 2.38                   | 79.38 $\pm$ 1.79  |
| eps    | 0   | <b>89.86 <math>\pm</math> 2.05</b> | 74.66 $\pm$ 0.68 | 84.02 $\pm$ 0.34                   | 70.37 $\pm$ 3.22 | <b>84.68 <math>\pm</math> 7.8</b>  | 60.36 $\pm$ 1.56                   | 75.68 $\pm$ 4.68                   | 41.44 $\pm$ 6.24  |
|        | 1   | <b>91.03 <math>\pm</math> 1.69</b> | 87.91 $\pm$ 0.68 | 89.08 $\pm$ 1.22                   | 82.46 $\pm$ 0.58 | <b>89.19 <math>\pm</math> 4.68</b> | 73.87 $\pm$ 1.56                   | 76.58 $\pm$ 1.56                   | 71.17 $\pm$ 4.13  |
|        | 5   | <b>87.72 <math>\pm</math> 1.55</b> | 86.55 $\pm$ 1.17 | 86.55 $\pm$ 1.55                   | 79.92 $\pm$ 1.88 | <b>89.19 <math>\pm</math> 5.41</b> | 74.77 $\pm$ 8.26                   | 77.48 $\pm$ 1.56                   | 68.47 $\pm$ 10.92 |
|        | 10  | <b>88.3 <math>\pm</math> 0.58</b>  | 86.94 $\pm$ 1.35 | 83.24 $\pm$ 1.35                   | 78.75 $\pm$ 2.36 | <b>88.29 <math>\pm</math> 3.12</b> | 74.77 $\pm$ 3.12                   | 75.68 $\pm$ 2.7                    | 69.37 $\pm$ 7.8   |
| sales  | 0   | <b>93.45 <math>\pm</math> 0.2</b>  | 77.97 $\pm$ 1.48 | 88.47 $\pm$ 1.89                   | 78.08 $\pm$ 2.4  | 89.28 $\pm$ 0.89                   | 75.83 $\pm$ 0.34                   | <b>89.86 <math>\pm</math> 0.68</b> | 54.58 $\pm$ 1.35  |
|        | 1   | <b>92.99 <math>\pm</math> 1.37</b> | 90.28 $\pm$ 0.2  | 91.41 $\pm$ 1.19                   | 86.78 $\pm$ 1.55 | 90.64 $\pm$ 1.17                   | 89.28 $\pm$ 2.05                   | <b>90.84 <math>\pm</math> 0.34</b> | 84.41 $\pm$ 2.21  |
|        | 5   | 92.09 $\pm$ 0.71                   | 90.62 $\pm$ 0.98 | <b>92.32 <math>\pm</math> 1.04</b> | 84.18 $\pm$ 1.09 | <b>90.84 <math>\pm</math> 1.47</b> | 89.67 $\pm$ 1.79                   | 89.47 $\pm$ 0.58                   | 82.26 $\pm$ 2.36  |
|        | 10  | <b>93.33 <math>\pm</math> 0.71</b> | 90.51 $\pm$ 0.34 | 91.41 $\pm$ 1.28                   | 84.41 $\pm$ 2.9  | 89.67 $\pm$ 0.89                   | <b>89.86 <math>\pm</math> 1.22</b> | 89.08 $\pm$ 1.47                   | 83.24 $\pm$ 0.34  |

Table S7: Mean accuracy (% ,  $\pm$  standard deviation) of LLMs on the ECT and SEC datasets, evaluated using the semantically most similar few-shot examples under No Transcript without Chain-of-Thought (CoT) prompting. For each dataset, the highest score within each row is presented in bold. Results are averaged over three independent runs.

| Target | $k$ | ECT Data                           |                                   |                                    |                  | SEC Data                           |                                    |                  |                  |
|--------|-----|------------------------------------|-----------------------------------|------------------------------------|------------------|------------------------------------|------------------------------------|------------------|------------------|
|        |     | GPT-4.1-Mini                       | Gemma3:27B                        | Llama3.3:70B                       | Mistral:24B      | GPT-4.1-Mini                       | Gemma3:24B                         | Llama3.3:70B     | Mistral:24B      |
| debt   | 0   | 85.57 $\pm$ 1.79                   | <b>87.29 <math>\pm</math> 0.6</b> | 84.19 $\pm$ 2.15                   | 78.69 $\pm$ 4.65 | <b>84.88 <math>\pm</math> 1.19</b> | 75.6 $\pm$ 0.6                     | 76.29 $\pm$ 1.79 | 53.26 $\pm$ 3.31 |
|        | 1   | 83.85 $\pm$ 0.6                    | 85.22 $\pm$ 0.6                   | <b>85.57 <math>\pm</math> 2.73</b> | 79.73 $\pm$ 4.29 | <b>83.51 <math>\pm</math> 1.79</b> | 78.35 $\pm$ 1.79                   | 75.95 $\pm$ 1.19 | 58.08 $\pm$ 2.59 |
|        | 5   | 80.76 $\pm$ 0.6                    | <b>86.25 <math>\pm</math> 0.6</b> | 84.54 $\pm$ 2.73                   | 77.32 $\pm$ 1.03 | <b>82.82 <math>\pm</math> 0.6</b>  | 74.91 $\pm$ 1.57                   | 79.73 $\pm$ 2.15 | 62.89 $\pm$ 2.06 |
|        | 10  | 83.16 $\pm$ 2.15                   | <b>85.22 <math>\pm</math> 0.6</b> | 83.16 $\pm$ 1.57                   | 80.07 $\pm$ 2.59 | <b>84.19 <math>\pm</math> 0.6</b>  | 78.01 $\pm$ 0.6                    | 73.54 $\pm$ 0.6  | 61.51 $\pm$ 1.57 |
| eps    | 0   | <b>88.89 <math>\pm</math> 1.01</b> | 82.26 $\pm$ 0.34                  | 83.63 $\pm$ 1.01                   | 77.0 $\pm$ 0.34  | <b>81.98 <math>\pm</math> 1.56</b> | 71.17 $\pm$ 1.56                   | 75.68 $\pm$ 0.0  | 53.15 $\pm$ 5.63 |
|        | 1   | <b>88.3 <math>\pm</math> 1.01</b>  | 84.99 $\pm$ 0.68                  | 87.13 $\pm$ 2.03                   | 77.58 $\pm$ 2.21 | <b>79.28 <math>\pm</math> 3.12</b> | 68.47 $\pm$ 1.56                   | 72.97 $\pm$ 0.0  | 58.56 $\pm$ 1.56 |
|        | 5   | <b>87.33 <math>\pm</math> 0.89</b> | 84.8 $\pm$ 0.58                   | 87.13 $\pm$ 3.83                   | 79.73 $\pm$ 0.89 | <b>77.48 <math>\pm</math> 1.56</b> | 66.67 $\pm$ 1.56                   | 69.37 $\pm$ 6.8  | 60.36 $\pm$ 1.56 |
|        | 10  | <b>87.13 <math>\pm</math> 0.58</b> | 86.55 $\pm$ 0.0                   | <b>87.13 <math>\pm</math> 0.58</b> | 78.36 $\pm$ 1.01 | <b>80.18 <math>\pm</math> 1.56</b> | 67.57 $\pm$ 0.0                    | 73.87 $\pm$ 4.13 | 55.86 $\pm$ 8.69 |
| sales  | 0   | <b>92.09 <math>\pm</math> 0.52</b> | 88.7 $\pm$ 0.2                    | 85.88 $\pm$ 1.67                   | 79.1 $\pm$ 0.2   | <b>91.81 <math>\pm</math> 0.58</b> | 91.62 $\pm$ 0.89                   | 90.84 $\pm$ 0.34 | 77.39 $\pm$ 1.88 |
|        | 1   | <b>93.33 <math>\pm</math> 0.2</b>  | 88.7 $\pm$ 0.52                   | 90.73 $\pm$ 1.6                    | 82.15 $\pm$ 1.67 | <b>94.93 <math>\pm</math> 0.34</b> | 93.96 $\pm$ 0.68                   | 89.86 $\pm$ 2.94 | 82.85 $\pm$ 2.76 |
|        | 5   | <b>92.32 <math>\pm</math> 0.39</b> | 87.46 $\pm$ 0.0                   | 88.59 $\pm$ 2.74                   | 83.28 $\pm$ 1.41 | <b>91.81 <math>\pm</math> 0.58</b> | <b>91.81 <math>\pm</math> 0.58</b> | 89.08 $\pm$ 3.0  | 80.31 $\pm$ 2.05 |
|        | 10  | <b>92.2 <math>\pm</math> 0.34</b>  | 88.7 $\pm$ 0.52                   | 89.38 $\pm$ 0.85                   | 82.82 $\pm$ 3.15 | <b>93.37 <math>\pm</math> 0.68</b> | 93.18 $\pm$ 0.34                   | 90.45 $\pm$ 0.34 | 83.24 $\pm$ 0.34 |

Table S8: Mean accuracy (% ,  $\pm$  standard deviation) of LLMs on the ECT and SEC datasets, evaluated using the semantically most similar few-shot examples under No Transcript with Chain-of-Thought (CoT) prompting conditions. For each dataset, the highest score within each row is presented in bold. Results are averaged over three independent runs.

| Target | $k$ | ECT Data                           |                                    |                                    |                  | SEC Data                           |                                    |                                    |                   |
|--------|-----|------------------------------------|------------------------------------|------------------------------------|------------------|------------------------------------|------------------------------------|------------------------------------|-------------------|
|        |     | GPT-4.1-Mini                       | Gemma3:27B                         | Llama3.3:70B                       | Mistral:24B      | GPT-4.1-Mini                       | Gemma3:24B                         | Llama3.3:70B                       | Mistral:24B       |
| debt   | 0   | 81.79 $\pm$ 3.15                   | 72.16 $\pm$ 4.12                   | <b>85.22 <math>\pm</math> 1.19</b> | 78.69 $\pm$ 2.59 | <b>82.82 <math>\pm</math> 1.57</b> | 63.57 $\pm$ 1.19                   | 80.07 $\pm$ 2.38                   | 75.6 $\pm$ 3.62   |
|        | 1   | <b>85.57 <math>\pm</math> 2.73</b> | 84.54 $\pm$ 1.79                   | 84.88 $\pm$ 2.15                   | 76.98 $\pm$ 1.19 | <b>85.57 <math>\pm</math> 2.73</b> | 84.19 $\pm$ 2.38                   | 84.54 $\pm$ 2.06                   | 74.57 $\pm$ 1.19  |
|        | 5   | <b>84.88 <math>\pm</math> 2.59</b> | 81.44 $\pm$ 2.06                   | 80.07 $\pm$ 1.19                   | 78.35 $\pm$ 1.03 | <b>89.35 <math>\pm</math> 2.15</b> | 85.91 $\pm$ 2.15                   | 87.29 $\pm$ 2.15                   | 70.1 $\pm$ 4.49   |
|        | 10  | <b>87.97 <math>\pm</math> 2.15</b> | 85.57 $\pm$ 1.79                   | 82.13 $\pm$ 1.57                   | 76.63 $\pm$ 2.15 | <b>88.32 <math>\pm</math> 2.38</b> | 83.85 $\pm$ 1.57                   | 82.47 $\pm$ 3.09                   | 79.38 $\pm$ 5.36  |
| eps    | 0   | <b>80.51 <math>\pm</math> 3.0</b>  | 53.02 $\pm$ 2.64                   | 80.12 $\pm$ 2.03                   | 78.36 $\pm$ 1.75 | <b>86.49 <math>\pm</math> 2.7</b>  | 37.84 $\pm$ 5.41                   | 80.18 $\pm$ 4.13                   | 63.06 $\pm$ 6.24  |
|        | 1   | <b>87.52 <math>\pm</math> 0.34</b> | 87.33 $\pm$ 1.69                   | 87.13 $\pm$ 0.58                   | 79.53 $\pm$ 1.75 | <b>92.79 <math>\pm</math> 3.12</b> | 82.88 $\pm$ 4.13                   | 82.88 $\pm$ 3.12                   | 74.77 $\pm$ 5.63  |
|        | 5   | 85.58 $\pm$ 0.89                   | 84.6 $\pm$ 1.35                    | <b>86.74 <math>\pm</math> 0.68</b> | 79.73 $\pm$ 2.05 | <b>88.29 <math>\pm</math> 6.8</b>  | 78.38 $\pm$ 2.7                    | 83.78 $\pm$ 2.7                    | 68.47 $\pm$ 11.25 |
|        | 10  | 84.6 $\pm$ 0.89                    | <b>86.35 <math>\pm</math> 0.89</b> | 85.96 $\pm$ 2.92                   | 79.92 $\pm$ 2.43 | <b>90.09 <math>\pm</math> 4.13</b> | 72.07 $\pm$ 3.12                   | 77.48 $\pm$ 4.13                   | 60.36 $\pm$ 1.56  |
| sales  | 0   | 77.85 $\pm$ 5.45                   | 59.77 $\pm$ 2.31                   | <b>88.59 <math>\pm</math> 0.52</b> | 83.05 $\pm$ 1.02 | 86.74 $\pm$ 2.21                   | 63.35 $\pm$ 1.79                   | <b>89.28 <math>\pm</math> 0.89</b> | 85.19 $\pm$ 0.89  |
|        | 1   | <b>92.66 <math>\pm</math> 0.85</b> | 88.93 $\pm$ 0.2                    | 90.06 $\pm$ 1.28                   | 87.68 $\pm$ 1.87 | 93.37 $\pm$ 1.22                   | <b>95.71 <math>\pm</math> 0.34</b> | 94.54 $\pm$ 0.34                   | 90.45 $\pm$ 1.22  |
|        | 5   | <b>92.09 <math>\pm</math> 0.85</b> | 90.4 $\pm$ 1.67                    | 89.94 $\pm$ 0.39                   | 85.65 $\pm$ 1.37 | 92.79 $\pm$ 2.05                   | <b>94.15 <math>\pm</math> 2.11</b> | 92.59 $\pm$ 0.89                   | 85.96 $\pm$ 2.03  |
|        | 10  | <b>92.43 <math>\pm</math> 0.39</b> | 90.73 $\pm$ 1.09                   | 89.72 $\pm$ 0.85                   | 86.89 $\pm$ 0.52 | 91.81 $\pm$ 1.01                   | <b>95.13 <math>\pm</math> 0.89</b> | 92.01 $\pm$ 2.94                   | 85.77 $\pm$ 1.22  |

Table S9: Mean accuracy (% ,  $\pm$  standard deviation) of LLMs on the ECT and SEC datasets, evaluated using the semantically most similar few-shot examples under Full Transcript prompting without Chain-of-Thought (CoT). For each dataset, the highest score within each row is presented in bold. Results are averaged over three independent runs.

| Target | $k$ | ECT Data                           |                  |                  |                  | SEC Data                           |                  |                  |                  |
|--------|-----|------------------------------------|------------------|------------------|------------------|------------------------------------|------------------|------------------|------------------|
|        |     | GPT-4.1-Mini                       | Gemma3:27B       | Llama3.3:70B     | Mistral:24B      | GPT-4.1-Mini                       | Gemma3:24B       | Llama3.3:70B     | Mistral:24B      |
| debt   | 0   | <b>91.41 <math>\pm</math> 1.57</b> | 84.54 $\pm$ 1.79 | 88.32 $\pm$ 1.57 | 39.52 $\pm$ 2.98 | <b>82.47 <math>\pm</math> 1.03</b> | 58.42 $\pm$ 2.59 | 51.89 $\pm$ 2.15 | 24.4 $\pm$ 1.57  |
|        | 1   | <b>89.35 <math>\pm</math> 1.19</b> | 80.41 $\pm$ 1.79 | 84.54 $\pm$ 2.73 | 58.76 $\pm$ 1.03 | <b>79.73 <math>\pm</math> 1.57</b> | 68.04 $\pm$ 2.73 | 61.86 $\pm$ 2.06 | 45.36 $\pm$ 2.06 |
|        | 5   | <b>89.0 <math>\pm</math> 1.19</b>  | 80.41 $\pm$ 1.03 | 82.47 $\pm$ 3.09 | 64.95 $\pm$ 2.06 | <b>79.73 <math>\pm</math> 0.6</b>  | 67.7 $\pm$ 2.38  | 65.29 $\pm$ 1.19 | 51.89 $\pm$ 2.38 |
|        | 10  | <b>85.91 <math>\pm</math> 1.57</b> | 81.44 $\pm$ 1.03 | 82.47 $\pm$ 3.72 | 61.17 $\pm$ 11.5 | <b>80.76 <math>\pm</math> 1.57</b> | 67.01 $\pm$ 1.03 | 62.2 $\pm$ 2.15  | 52.58 $\pm$ 1.03 |
| eps    | 0   | <b>87.52 <math>\pm</math> 0.68</b> | 86.35 $\pm$ 0.89 | 85.77 $\pm$ 3.22 | 62.18 $\pm$ 1.88 | <b>81.08 <math>\pm</math> 0.0</b>  | 66.67 $\pm$ 1.56 | 63.06 $\pm$ 1.56 | 42.34 $\pm$ 4.13 |
|        | 1   | <b>91.81 <math>\pm</math> 0.58</b> | 87.33 $\pm$ 0.34 | 85.77 $\pm$ 2.05 | 67.64 $\pm$ 2.36 | <b>84.68 <math>\pm</math> 1.56</b> | 71.17 $\pm$ 1.56 | 67.57 $\pm$ 0.0  | 48.65 $\pm$ 2.7  |
|        | 5   | <b>91.03 <math>\pm</math> 0.34</b> | 85.96 $\pm$ 0.0  | 84.8 $\pm$ 2.55  | 70.57 $\pm$ 3.22 | <b>81.08 <math>\pm</math> 2.7</b>  | 72.97 $\pm$ 2.7  | 67.57 $\pm$ 2.7  | 54.95 $\pm$ 4.13 |
|        | 10  | <b>90.84 <math>\pm</math> 0.89</b> | 84.02 $\pm$ 1.22 | 84.8 $\pm$ 1.55  | 69.2 $\pm$ 1.47  | <b>81.98 <math>\pm</math> 3.12</b> | 73.87 $\pm$ 1.56 | 67.57 $\pm$ 0.0  | 55.86 $\pm$ 1.56 |
| sales  | 0   | <b>92.99 <math>\pm</math> 0.52</b> | 89.38 $\pm$ 1.09 | 88.47 $\pm$ 2.71 | 62.37 $\pm$ 1.79 | <b>91.42 <math>\pm</math> 0.89</b> | 86.55 $\pm$ 1.55 | 88.11 $\pm$ 2.21 | 60.43 $\pm$ 3.0  |
|        | 1   | <b>94.01 <math>\pm</math> 0.2</b>  | 88.02 $\pm$ 0.52 | 88.93 $\pm$ 2.21 | 65.88 $\pm$ 4.58 | <b>93.76 <math>\pm</math> 0.34</b> | 86.94 $\pm$ 1.79 | 90.25 $\pm$ 1.79 | 77.19 $\pm$ 1.75 |
|        | 5   | <b>93.79 <math>\pm</math> 0.2</b>  | 89.04 $\pm$ 0.85 | 90.28 $\pm$ 1.37 | 72.09 $\pm$ 1.19 | <b>91.03 <math>\pm</math> 1.47</b> | 87.13 $\pm$ 2.11 | 88.3 $\pm$ 2.11  | 76.22 $\pm$ 2.88 |
|        | 10  | <b>93.77 <math>\pm</math> 0.22</b> | 89.49 $\pm$ 0.59 | 89.94 $\pm$ 1.41 | 69.04 $\pm$ 0.85 | <b>89.86 <math>\pm</math> 0.34</b> | 87.72 $\pm$ 2.55 | 86.94 $\pm$ 2.21 | 74.07 $\pm$ 1.69 |

Table S10: Mean accuracy (% ,  $\pm$  standard deviation) of LLMs on the ECT and SEC datasets, evaluated using the semantically most similar few-shot examples under Full Transcript with Chain-of-Thought (CoT) prompting conditions. For each dataset, the highest score within each row is presented in bold. Results are averaged over three independent runs.

| Target | $k$ | ECT Data                           |                  |                                    |                  | SEC Data                           |                                    |                  |                  |
|--------|-----|------------------------------------|------------------|------------------------------------|------------------|------------------------------------|------------------------------------|------------------|------------------|
|        |     | GPT-4.1-Mini                       | Gemma3:27B       | Llama3.3:70B                       | Mistral:24B      | GPT-4.1-Mini                       | Gemma3:24B                         | Llama3.3:70B     | Mistral:24B      |
| debt   | 0   | <b>87.97 <math>\pm</math> 4.87</b> | 74.91 $\pm$ 4.17 | 84.19 $\pm$ 1.57                   | 50.86 $\pm$ 5.86 | <b>75.6 <math>\pm</math> 0.6</b>   | 68.04 $\pm$ 3.57                   | 74.91 $\pm$ 2.15 | 36.77 $\pm$ 5.68 |
|        | 1   | <b>91.75 <math>\pm</math> 1.03</b> | 81.79 $\pm$ 2.15 | 84.19 $\pm$ 1.57                   | 79.73 $\pm$ 3.62 | <b>86.94 <math>\pm</math> 2.15</b> | 83.51 $\pm$ 1.79                   | 84.54 $\pm$ 2.06 | 76.98 $\pm$ 2.59 |
|        | 5   | <b>90.38 <math>\pm</math> 0.6</b>  | 82.82 $\pm$ 1.19 | 84.88 $\pm$ 2.15                   | 80.07 $\pm$ 2.15 | <b>89.35 <math>\pm</math> 1.57</b> | 83.51 $\pm$ 1.03                   | 83.85 $\pm$ 2.59 | 76.98 $\pm$ 3.31 |
|        | 10  | <b>91.07 <math>\pm</math> 1.57</b> | 85.22 $\pm$ 1.57 | 85.57 $\pm$ 3.09                   | 80.07 $\pm$ 3.62 | <b>86.94 <math>\pm</math> 1.57</b> | 83.85 $\pm$ 0.6                    | 84.19 $\pm$ 5.68 | 80.07 $\pm$ 4.17 |
| eps    | 0   | <b>86.55 <math>\pm</math> 1.55</b> | 84.6 $\pm$ 1.35  | 84.6 $\pm$ 0.89                    | 59.65 $\pm$ 2.55 | <b>79.28 <math>\pm</math> 4.13</b> | 63.96 $\pm$ 4.13                   | 72.97 $\pm$ 2.7  | 46.85 $\pm$ 6.24 |
|        | 1   | <b>90.84 <math>\pm</math> 0.68</b> | 88.3 $\pm$ 0.58  | 85.38 $\pm$ 0.58                   | 80.7 $\pm$ 1.55  | <b>91.89 <math>\pm</math> 2.7</b>  | 81.98 $\pm$ 1.56                   | 75.68 $\pm$ 2.7  | 73.87 $\pm$ 1.56 |
|        | 5   | <b>89.86 <math>\pm</math> 1.35</b> | 88.5 $\pm$ 0.89  | 84.8 $\pm$ 1.55                    | 84.21 $\pm$ 1.17 | <b>83.78 <math>\pm</math> 2.7</b>  | 81.08 $\pm$ 2.7                    | 77.48 $\pm$ 1.56 | 66.67 $\pm$ 8.26 |
|        | 10  | <b>90.45 <math>\pm</math> 0.89</b> | 87.72 $\pm$ 1.17 | 84.6 $\pm$ 0.89                    | 80.51 $\pm$ 3.57 | <b>85.59 <math>\pm</math> 1.56</b> | 75.68 $\pm$ 2.7                    | 75.68 $\pm$ 2.7  | 64.86 $\pm$ 2.7  |
| sales  | 0   | 89.27 $\pm$ 1.99                   | 81.58 $\pm$ 1.19 | <b>91.86 <math>\pm</math> 2.12</b> | 64.52 $\pm$ 2.92 | <b>90.25 <math>\pm</math> 3.0</b>  | 66.47 $\pm$ 2.64                   | 89.08 $\pm$ 0.68 | 60.43 $\pm$ 4.23 |
|        | 1   | <b>95.48 <math>\pm</math> 0.78</b> | 90.96 $\pm$ 1.04 | 90.4 $\pm$ 0.52                    | 87.68 $\pm$ 2.54 | 94.15 $\pm$ 2.34                   | <b>95.32 <math>\pm</math> 0.58</b> | 90.25 $\pm$ 1.47 | 91.23 $\pm$ 0.58 |
|        | 5   | <b>93.9 <math>\pm</math> 0.34</b>  | 90.4 $\pm$ 0.52  | 90.85 $\pm$ 1.36                   | 85.88 $\pm$ 1.28 | 93.57 $\pm$ 1.17                   | <b>94.35 <math>\pm</math> 0.68</b> | 88.69 $\pm$ 1.22 | 86.55 $\pm$ 1.55 |
|        | 10  | <b>93.33 <math>\pm</math> 0.85</b> | 91.19 $\pm$ 0.68 | 90.51 $\pm$ 0.68                   | 87.23 $\pm$ 1.28 | <b>93.76 <math>\pm</math> 0.68</b> | 93.18 $\pm$ 0.34                   | 87.72 $\pm$ 1.55 | 84.6 $\pm$ 1.22  |

Table S11: Mean accuracy (% ,  $\pm$  standard deviation) of LLMs on the ECT and SEC datasets, evaluated using the semantically most similar few-shot examples under the Summarized Transcript setting without Chain-of-Thought (CoT) reasoning. For each dataset, the highest score within each row is presented in bold. Results are averaged over three independent runs.

| Target | $k$ | ECT Data                           |                  |                  |                  | SEC Data                           |                  |                                    |                  |
|--------|-----|------------------------------------|------------------|------------------|------------------|------------------------------------|------------------|------------------------------------|------------------|
|        |     | GPT-4.1-Mini                       | Gemma3:27B       | Llama3.3:70B     | Mistral:24B      | GPT-4.1-Mini                       | Gemma3:24B       | Llama3.3:70B                       | Mistral:24B      |
| debt   | 0   | <b>89.35 <math>\pm</math> 0.6</b>  | 88.32 $\pm$ 0.6  | 84.88 $\pm$ 3.31 | 74.23 $\pm$ 4.72 | <b>82.82 <math>\pm</math> 1.57</b> | 71.82 $\pm$ 0.6  | 76.29 $\pm$ 2.06                   | 20.27 $\pm$ 0.6  |
|        | 1   | <b>89.0 <math>\pm</math> 1.57</b>  | 86.6 $\pm$ 1.03  | 85.91 $\pm$ 3.62 | 75.26 $\pm$ 1.79 | <b>82.47 <math>\pm</math> 1.03</b> | 73.54 $\pm$ 0.6  | 78.35 $\pm$ 1.79                   | 44.33 $\pm$ 1.03 |
|        | 5   | <b>87.29 <math>\pm</math> 0.6</b>  | 84.54 $\pm$ 1.03 | 83.51 $\pm$ 4.49 | 69.76 $\pm$ 2.15 | <b>82.82 <math>\pm</math> 0.6</b>  | 71.48 $\pm$ 0.6  | 81.79 $\pm$ 1.57                   | 47.77 $\pm$ 2.38 |
|        | 10  | <b>89.0 <math>\pm</math> 0.6</b>   | 83.85 $\pm$ 1.57 | 85.22 $\pm$ 2.15 | 67.01 $\pm$ 1.03 | <b>82.47 <math>\pm</math> 0.0</b>  | 69.76 $\pm$ 3.31 | 76.98 $\pm$ 3.31                   | 49.83 $\pm$ 2.59 |
| eps    | 0   | <b>88.89 <math>\pm</math> 0.58</b> | 84.6 $\pm$ 1.47  | 84.8 $\pm$ 2.11  | 70.57 $\pm$ 1.79 | <b>79.28 <math>\pm</math> 3.12</b> | 71.17 $\pm$ 1.56 | 68.47 $\pm$ 3.12                   | 46.85 $\pm$ 6.8  |
|        | 1   | <b>88.89 <math>\pm</math> 1.17</b> | 85.38 $\pm$ 0.0  | 84.02 $\pm$ 3.22 | 70.96 $\pm$ 2.64 | <b>85.59 <math>\pm</math> 4.13</b> | 70.27 $\pm$ 2.7  | 68.47 $\pm$ 3.12                   | 50.45 $\pm$ 3.12 |
|        | 5   | <b>89.28 <math>\pm</math> 0.89</b> | 87.33 $\pm$ 0.34 | 84.6 $\pm$ 2.43  | 70.57 $\pm$ 2.76 | <b>83.78 <math>\pm</math> 2.7</b>  | 72.97 $\pm$ 4.68 | 72.07 $\pm$ 3.12                   | 60.36 $\pm$ 1.56 |
|        | 10  | <b>89.08 <math>\pm</math> 0.34</b> | 87.13 $\pm$ 0.0  | 85.19 $\pm$ 1.35 | 73.29 $\pm$ 2.21 | <b>83.78 <math>\pm</math> 0.0</b>  | 74.77 $\pm$ 4.13 | 69.37 $\pm$ 1.56                   | 54.95 $\pm$ 6.24 |
| sales  | 0   | <b>92.88 <math>\pm</math> 0.34</b> | 90.17 $\pm$ 0.68 | 89.94 $\pm$ 2.07 | 71.86 $\pm$ 0.68 | <b>91.81 <math>\pm</math> 0.58</b> | 88.11 $\pm$ 1.22 | 91.23 $\pm$ 1.55                   | 44.44 $\pm$ 1.55 |
|        | 1   | <b>93.11 <math>\pm</math> 0.2</b>  | 89.94 $\pm$ 0.39 | 88.47 $\pm$ 2.03 | 76.05 $\pm$ 0.52 | <b>93.76 <math>\pm</math> 0.68</b> | 91.23 $\pm$ 0.58 | 89.47 $\pm$ 2.92                   | 65.69 $\pm$ 3.8  |
|        | 5   | <b>93.45 <math>\pm</math> 0.39</b> | 88.93 $\pm$ 0.2  | 89.72 $\pm$ 1.6  | 73.33 $\pm$ 1.28 | 92.59 $\pm$ 0.34                   | 89.67 $\pm$ 0.89 | <b>92.79 <math>\pm</math> 1.22</b> | 69.79 $\pm$ 1.22 |
|        | 10  | <b>92.77 <math>\pm</math> 0.85</b> | 89.72 $\pm$ 0.85 | 88.02 $\pm$ 1.41 | 66.33 $\pm$ 3.62 | <b>92.01 <math>\pm</math> 0.34</b> | 90.06 $\pm$ 1.55 | 89.08 $\pm$ 0.34                   | 72.32 $\pm$ 2.64 |

Table S12: Mean accuracy (% ,  $\pm$  standard deviation) of LLMs on the ECT and SEC datasets, evaluated using the semantically most similar few-shot examples under Summarized Transcript with Chain-of-Thought (CoT) prompting conditions. For each dataset, the highest score within each row is presented in bold. Results are averaged over three independent runs.

| Target | $k$ | ECT Data                           |                  |                                    |                  | SEC Data                           |                                    |                                    |                   |
|--------|-----|------------------------------------|------------------|------------------------------------|------------------|------------------------------------|------------------------------------|------------------------------------|-------------------|
|        |     | GPT-4.1-Mini                       | Gemma3:27B       | Llama3.3:70B                       | Mistral:24B      | GPT-4.1-Mini                       | Gemma3:24B                         | Llama3.3:70B                       | Mistral:24B       |
| debt   | 0   | <b>88.32 <math>\pm</math> 2.59</b> | 80.07 $\pm$ 2.98 | 86.25 $\pm$ 3.62                   | 75.95 $\pm$ 1.57 | 79.73 $\pm$ 1.19                   | 69.76 $\pm$ 3.15                   | <b>80.76 <math>\pm</math> 0.6</b>  | 35.74 $\pm$ 0.6   |
|        | 1   | <b>88.32 <math>\pm</math> 2.15</b> | 81.44 $\pm$ 0.0  | 85.22 $\pm$ 1.57                   | 75.26 $\pm$ 3.09 | <b>86.25 <math>\pm</math> 1.19</b> | 84.54 $\pm$ 1.79                   | 84.88 $\pm$ 1.19                   | 80.07 $\pm$ 4.87  |
|        | 5   | <b>90.03 <math>\pm</math> 2.15</b> | 82.13 $\pm$ 0.6  | 84.54 $\pm$ 2.06                   | 80.07 $\pm$ 2.98 | <b>89.35 <math>\pm</math> 1.57</b> | 85.57 $\pm$ 1.79                   | 85.57 $\pm$ 1.03                   | 72.85 $\pm$ 4.29  |
|        | 10  | <b>89.69 <math>\pm</math> 1.79</b> | 83.51 $\pm$ 1.03 | 85.91 $\pm$ 2.15                   | 78.69 $\pm$ 1.57 | <b>89.69 <math>\pm</math> 1.03</b> | 82.13 $\pm$ 2.59                   | 82.82 $\pm$ 3.31                   | 80.41 $\pm$ 2.06  |
| eps    | 0   | <b>87.91 <math>\pm</math> 1.22</b> | 74.07 $\pm$ 0.89 | 86.35 $\pm$ 0.89                   | 73.68 $\pm$ 3.26 | <b>88.29 <math>\pm</math> 1.56</b> | 59.46 $\pm$ 0.0                    | 70.27 $\pm$ 2.7                    | 45.95 $\pm$ 14.04 |
|        | 1   | <b>89.67 <math>\pm</math> 0.34</b> | 89.08 $\pm$ 2.76 | 86.94 $\pm$ 0.89                   | 79.14 $\pm$ 0.68 | <b>92.79 <math>\pm</math> 3.12</b> | 81.98 $\pm$ 1.56                   | 81.08 $\pm$ 2.7                    | 72.97 $\pm$ 2.7   |
|        | 5   | <b>90.25 <math>\pm</math> 1.69</b> | 88.11 $\pm$ 1.22 | 85.58 $\pm$ 2.21                   | 82.07 $\pm$ 0.34 | <b>91.89 <math>\pm</math> 0.0</b>  | 81.98 $\pm$ 3.12                   | 81.08 $\pm$ 2.7                    | 68.47 $\pm$ 4.13  |
|        | 10  | <b>89.47 <math>\pm</math> 0.58</b> | 85.96 $\pm$ 0.58 | 85.58 $\pm$ 1.79                   | 79.73 $\pm$ 1.22 | <b>87.39 <math>\pm</math> 1.56</b> | 80.18 $\pm$ 1.56                   | 80.18 $\pm$ 5.63                   | 68.47 $\pm$ 3.12  |
| sales  | 0   | <b>92.88 <math>\pm</math> 1.22</b> | 78.42 $\pm$ 0.78 | 88.47 $\pm$ 1.22                   | 78.87 $\pm$ 1.96 | 90.25 $\pm$ 0.89                   | 74.66 $\pm$ 0.34                   | <b>90.64 <math>\pm</math> 1.01</b> | 50.1 $\pm$ 1.35   |
|        | 1   | <b>93.22 <math>\pm</math> 0.68</b> | 91.07 $\pm$ 0.71 | 91.86 $\pm$ 0.59                   | 86.44 $\pm$ 1.89 | 94.15 $\pm$ 0.58                   | <b>96.69 <math>\pm</math> 0.68</b> | 93.96 $\pm$ 0.89                   | 88.89 $\pm$ 0.0   |
|        | 5   | <b>92.09 <math>\pm</math> 0.85</b> | 91.98 $\pm$ 0.39 | <b>92.09 <math>\pm</math> 1.04</b> | 85.2 $\pm$ 1.74  | 93.57 $\pm$ 0.58                   | <b>94.35 <math>\pm</math> 0.34</b> | 90.84 $\pm$ 0.89                   | 87.52 $\pm$ 2.64  |
|        | 10  | <b>92.54 <math>\pm</math> 0.9</b>  | 90.4 $\pm$ 1.28  | 90.17 $\pm$ 1.48                   | 84.97 $\pm$ 1.93 | <b>94.54 <math>\pm</math> 0.89</b> | 94.15 $\pm$ 1.55                   | 91.81 $\pm$ 1.55                   | 86.35 $\pm$ 3.33  |
